# Supplementary material for: Spontaneous Formation of Exceptional Points at the Onset of Magnetism
Source: arXiv:2207.05097 source file (2023-10-06)
Supplement: Supplementary file 1 [file supplemental.pdf]

# Supplemental material for: Spontaneous Formation of Exceptional Points at the Onset of Magnetism

L. Crippa,[1] G. Sangiovanni,[1] and J. C. Budich[2]

[1]*Institut für Theoretische Physik und Astrophysik and Würzburg-Dresden Cluster of Excellence ct.qmat, Universität Würzburg, 97074 Würzburg, Germany*

[2]*Institute of Theoretical Physics, Technische Universität Dresden and and Würzburg-Dresden Cluster of Excellence ct.qmat, 01062 Dresden, Germany*

**SURFACE HAMILTONIAN FORM**

We follow the derivation presented in reference [42] in the main text, discarding however higher-order terms. First, we introduce the Dirac matrices

$$\Gamma_1 = \sigma_z \otimes \tau_x, \quad \Gamma_2 = -\mathbb{I} \otimes \tau_y, \quad \Gamma_3 = \sigma_x \otimes \tau_x, \quad \Gamma_4 = \sigma_y \otimes \tau_x, \quad \Gamma_5 = \mathbb{I} \otimes \tau_z \tag{1}$$

(where $\sigma_i$ and $\tau_i$ act on the spin and orbital subspaces respectively) and determine the linearized form of the 3d BHZ Hamiltonian in the proximity of a bulk high-symmetry point, up to second order for $\sin k_i$ and $\cos k_i$. In our slab setup, we can write such a linearized Hamiltonian as a sum of an in-plane $H_{||}$ and a term $H_y$ containing the hopping along the finite direction. We than have

$$H_y = (\overline{M} + k_y^2)\Gamma_5 + \lambda \Gamma_2 k_y \tag{2}$$

and

$$H_{||} = k_{||}^2 \Gamma_5 + \lambda(\Gamma_1 k_x + \Gamma_3 k_z). \tag{3}$$

where $\overline{M}$ is not simply the BHZ mass parameter, but a constant term containing the lowest-order Taylor coefficients of the trigonometric function expansions and can hence be negative. Note that an additional minus sign can appear in front of the $k$ terms depending on which high-symmetry point we are linearizing the Hamiltonian around, without changing the spirit of the derivation. We will assume positive signs for the rest of this section. The presence of a boundary is accounted for by passing back to real space in the $y$ direction, substituting $k_y \to -i\partial_y$. Since $\Gamma_2$ and $\Gamma_5$ are both block-diagonal in spin space, the eigenstates of $H_y$ will be of the type

$$\Psi_\uparrow = [\psi_0, \mathbf{0}], \quad \Psi_\downarrow = [\mathbf{0}, \psi_0] \tag{4}$$

wher $\mathbf{0}$ is a 2-component null vector and $\psi_0$ is a 2-component vector which satisfies

$$\left[(\overline{M} - \partial_y^2)\tau_3 - i\lambda\tau_2\partial_z\right]\psi_0 = E\psi_0. \tag{5}$$

Assuming we are linearizing the Hamiltonian around a high-symmetry point where the surface states cross, in the presence of particle-hole symmetry we can enforce the zero-energy requirement for the surface states, thereby removing the right hand side term in Eq.(5). We then multiply the

left-hand side by $\tau_y$ and, considering as an ansatz an exponentially localized eigenstate of the type $\psi_0 = \phi e^{\Lambda y}$ we can recast Eq.(5) as

$$(\overline{M} - \Lambda^2)\tau_x \phi = \lambda \Lambda \phi \tag{6}$$

from which clearly $\phi$ has to be an eigenstate of $\tau_x$. We define $\tau_x \phi_\pm = \pm \phi_\pm$: from the considerations above, a general expression for $\psi_0$ reads

$$\psi_0 = (a e^{\Lambda_1 y} + b e^{\Lambda_2 y})\phi_+ + (c e^{-\Lambda_1 y} + d e^{-\Lambda_2 y})\phi_- \tag{7}$$

where

$$\Lambda_{1,2} = \frac{1}{2}\big( - \lambda \pm \sqrt{\lambda^2 + 4\overline{M}}.\big) \tag{8}$$

We can further simplify these expressions: from and the normalizability condition for $y > 0$, the surface state decays away from the border if $\Lambda_{1,2}$ is negative. Together with $\lambda > 0$, this implies $\overline{M} < 0$, which reflects the mass inversion in the topological gap. Keeping in mind the open boundary condition condition $\psi_0(0) = 0$, then, the expression for the eigenstate is simplified to read

$$\psi_0 = a(e^{\Lambda_1 y} - e^{\Lambda_2 y})\phi_+. \tag{9}$$

The decay length is given by

$$l = \max \frac{1}{|\mathrm{Re}\Lambda_{1,2}|} = \frac{1}{\left|\mathrm{Re}\Big( - \frac{\lambda + \sqrt{\lambda^2 + 4\overline{M}}}{2}\Big)\right|} \tag{10}$$

which puts in relation the values of spin-orbit coupling and topological mass. Finally, a form for the surface Hamiltonian can be written in the space of $\Psi = \mathrm{span}(\Psi_\uparrow, \Psi_\downarrow)$, remembering that, from the form of $\Psi$ given in Eq.(4), the following holds:

$$\langle \Psi | \Gamma_1 | \Psi \rangle = \sigma_z \alpha_1, \quad \langle \Psi | \Gamma_3 | \Psi \rangle = \sigma_x \alpha_1, \tag{11}$$

where $\alpha_1 = \langle \psi_0 | \tau_x | \psi_0 \rangle$. This justifies the expression for the surface Hamiltonian found in the main text, which to the lowest order in $k$ reads

$$H_{\mathrm{surf}} = \lambda \alpha_1 (\sigma_x k_z + \sigma_z k_x). \tag{12}$$

## SELF-ENERGY STRUCTURE AND NUMERICAL EFFECTS

Fig. 4 in the main text shows the effect of the finite-temperature DMFT self-energy $\Sigma(0)$ on the effective band dispersion of the system. It is interesting to note how the band dispersion is not symmetric, which is mostly evident from the plot of the imaginary part. In order to explain this fact, we briefly elaborate on the matrix structure of the self-energy and on numerical effects inherent to its calculation. Real-space DMFT is a solution method based on the assumption that only local many-body fluctuations are treated beyond the mean-field level. The inequivalent nature of the individual layers of the slab is fully taken into account through a single-particle Hamiltonian and the set of inequivalent, albeit site-local, self-energies. The latter are obtained solving the set of impurity problems, one for each (inequivalent) layer of the slab. In a hybrid representation that passes back to real space in the finite direction, the single-particle Hamiltonian of the slab can be written as

$$H_{\text{full}}(\mathbf{k}) = \begin{bmatrix} \boxed{H_1(\mathbf{k})} & T_{12} & 0 & 0 & \dots \\ T_{12}^{\dagger} & \boxed{H_2(\mathbf{k})} & T_{23} & 0 & \dots \\ 0 & T_{23}^{\dagger} & \boxed{H_3(\mathbf{k})} & T_{34} & \dots \\ 0 & 0 & T_{34}^{\dagger} & \boxed{H_4(\mathbf{k})} & \dots \\ \vdots & \vdots & \vdots & \vdots & \ddots \end{bmatrix} \tag{13}$$

where $H_i(\mathbf{k})$ is the in-plane Hamiltonian of each layer and $T_{ij}$ are the hopping terms between the layers. To apply the Real Space-DMFT method, we must operate both at the level of the full slab and of the individual layers: at the slab level, the relevant quantity to treat is the full local Green's function $G_{\text{loc}}$. This is built as

$$G_{\text{loc}}(i\omega) = \sum_{\mathbf{k}} \frac{1}{i\omega\mathbb{I} - H_{\text{full}}(\mathbf{k}) - \Sigma(i\omega)} \tag{14}$$

where $\Sigma$ is the self-energy which, because of its site-local nature, corresponds to the direct sum of layer-resolved self-energies $\Sigma = \bigoplus_i \Sigma_i$. Each $\Sigma_i$ is determined by solving a layer-by-layer appropriately defined effective impurity model, whose Hamiltonian replicates the local physics of each $H_i$ block in Eq.(13) and whose dynamical bath or Weiss field $\mathcal{G}_i$ carries information on the intra-layer hoppings $T_{ij}$. For each layer, the Weiss field is defined through the Dyson equation

$$\mathcal{G}_i^{-1} = \Sigma_i + \left[G_{\text{loc}}\big|_i\right]^{-1} \tag{15}$$

where the last term is obtained by inverting the $(N_{\text{orbital}} \cdot N_{\text{spin}}) \times (N_{\text{orbital}} \cdot N_{\text{spin}})$ block of $G_{\text{loc}}$ corresponding to the $i$-th layer. As a result, local correlation effects are fully accounted for, while the non-local ones are included at the mean-field (Hartree-Fock) level only.

Since the $H_i$ blocks only possess orbital-diagonal local components, one might expect that the relative self-energies $\Sigma_i$ would share the same property. This is however not the case and the reason is the orbital off-diagonal structure of the dynamical bath $\mathcal{G}_i^{-1}$ for sites at the border of the slab. The frequency dependence of the individual Weiss fields is a result of a matrix inversion involving the full $G_{\text{loc}}$ and is hence influenced by the structure of the full Hamiltonian, comprising the $T$ hopping blocks. The asymmetry between bulk and surface layers then reflects in different $\mathcal{G}_i^{-1}$. In particular, because of the absence of periodic boundary conditions along the finite dimension of the slab, some hopping processes such as $\boxed{\text{layer 1}} \xrightarrow{\lambda} \boxed{\text{layer 2}} \xrightarrow{t} \boxed{\text{layer 1}}$ are not compensated by equivalent ones in opposite directions. As a result, *dynamical* orbital off-diagonal elements in the Weiss field at the surface emerge, despite the local Hamiltonian of the corresponding sites being orbital-diagonal. Consequently, the self-consistence loop causes the self-energy of the surface layers to develop off-diagonal inter-orbital terms as well. These terms are, in general, quite noisy in QMC-DMFT and give rise to numerical imprecision. Being the off-diagonal components of the self-energy always at least one order of magnitude smaller than the diagonal ones, however, their error bar does not affect the overall picture. Further, as the exceptional points are, by definition, robust topological entities, they are not destroyed by such small perturbations.

The asymmetry in the eigenvalue dispersion of Fig. 4 is thus explained: in part, this is due to the aforementioned statistical inaccuracies, but its cause is rooted in the difference between the self-energies of the bulk and surface layers and in the presence of off-diagonal orbital components.

## EFFECTS OF FINITE SIZE ON THE EXCEPTIONAL POINTS

As discussed in the main text, the surface Hamiltonian outlined in the first part of this supplemental material is accurate provided the slab is thick enough so that surface states do not hybridize with each other. In Fig. 1 we show the real and imaginary parts of the eigenvalues of the effective Hamiltonian along the $k_z$ direction for different slab thicknesses, and the relative real space localization of the surface eigenstate in the finite slab direction. For thinner slabs, the surface

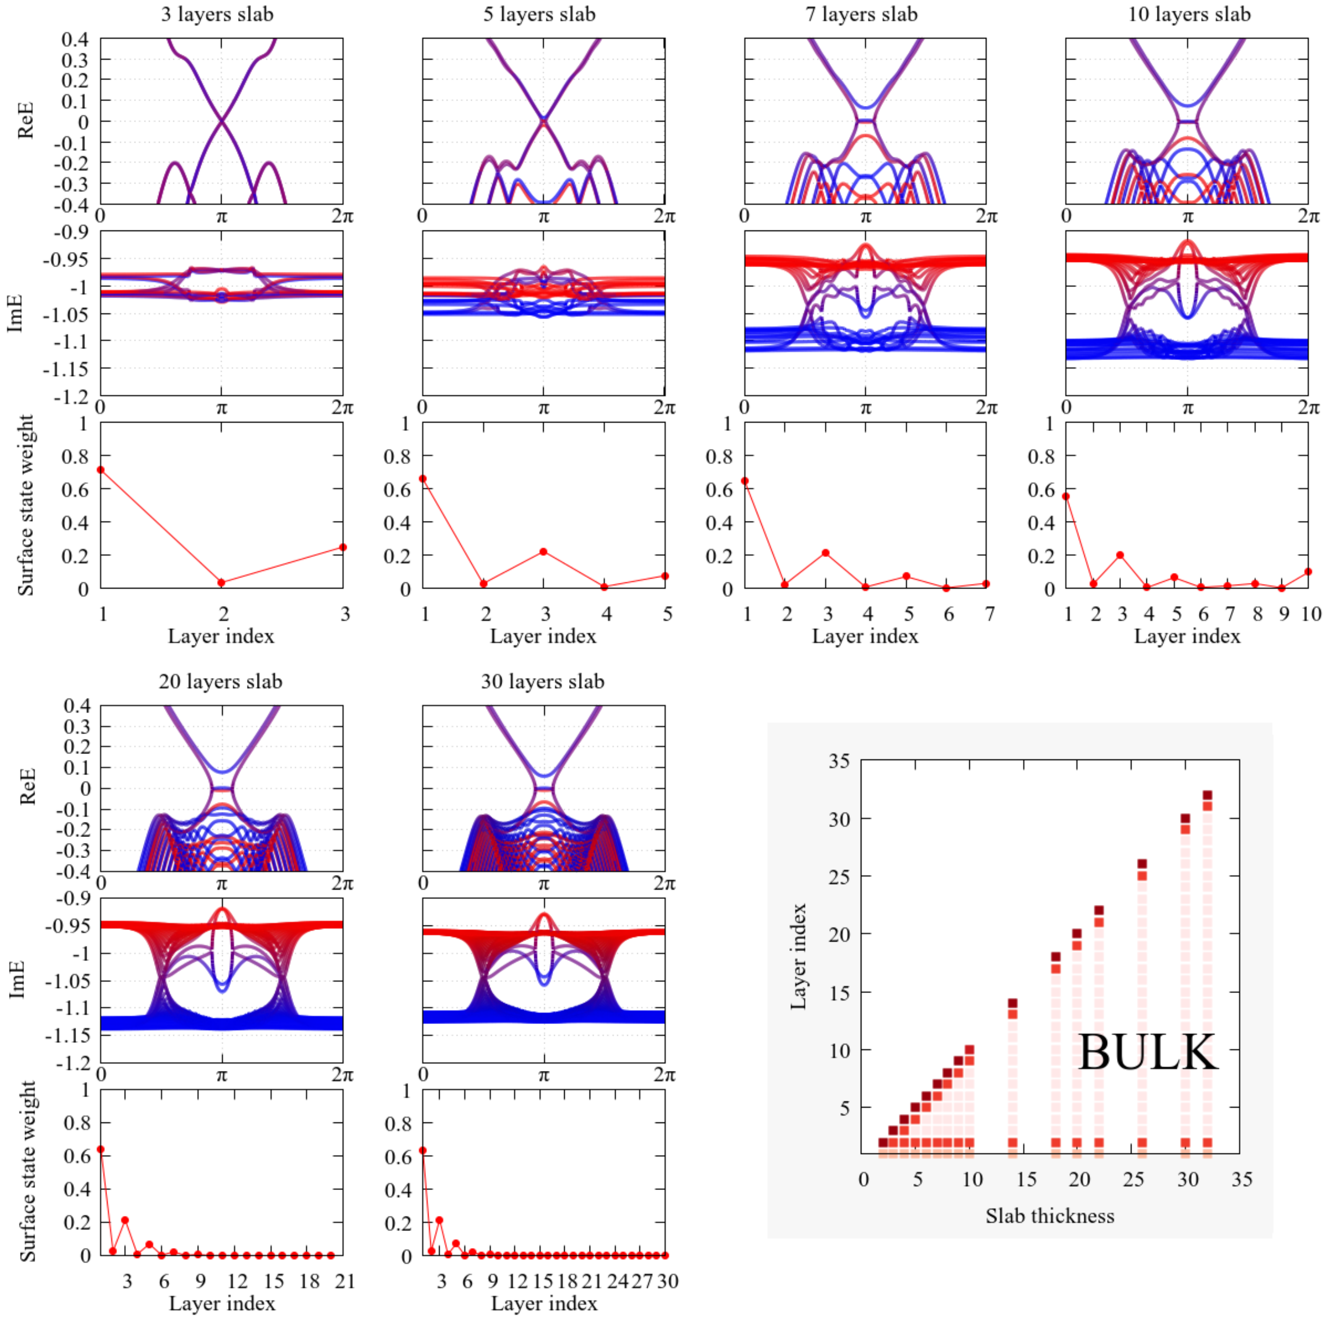


Figure 1. (color online) Real and imaginary part of the effective Hamiltonian eigenvalues along $k_z$, and surface eigenstate localization near the EPs for different thicknesses of the slab. The model parameters are $(U, U', J, T, \mu) = (13.0, 7.0, 6.0, 0.13, 2.00)$. The gap-closing points, as well as the square-root dispersion behavior emerging from them, are well defined above thickness 10. In the bottom-right shaded panel, layers that are equivalent for the purpose of DMFT are plotted in the same shade of red, for slabs of different thicknesses.

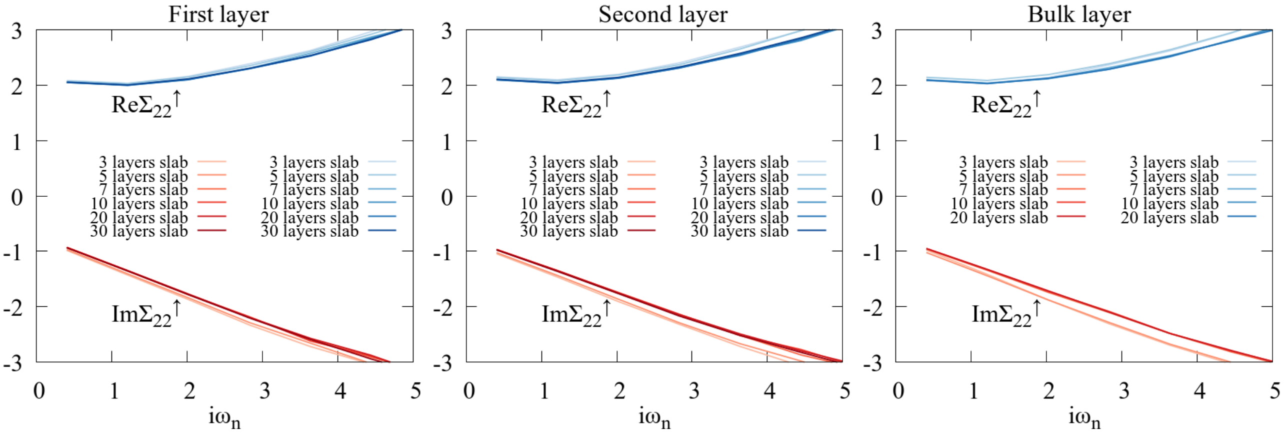


Figure 2. (color online) Real and imaginary part of the self-energy on the Matsubara axis for one orbital and spin, and various slab thicknesses. In the three panels, corresponding layers in the various geometries are compared. The bulk sites for very slim slabs are omitted.

eigenstate has sizeable spectral weight on both slab surfaces and in the bulk, and the magnetiztion is, moreover, too small to clearly incite the formation of the EPs. The concomitant degeneracies of real and imaginary parts of the band dispersions are therefore not well defined, and the imaginary part of the eigenvalues in particular shows peculiar oscillations. On the contrary for thicker slabs, and especially for more than 10 layers, the EPs become more and more clearly defined, and so is the associated square-root energy dispersion. This makes our choice of a 20-layer slab a good compromise between computational efficiency and surface Hamiltonian definiteness.

On the numerical front, a substantial computational time improvement in the real-space DMFT calculations can be achieved by only solving inequivalent impurity problems: indeed, for layers deep in the bulk of the slab, the associated local Green's functions become effectively identical, making the solution of all the relative impurity models redundant. In the bottom right shaded panel of Fig. 1 we plot the in various shades of red the layers whose local G is identical under a numerical threshold of $10^{-3}$. As it can be seen, already at thickness 6 the inner layers of the slab have equivalent local Green's function, and therefore entail identical DMFT self-energies. We explicitly compare the self-energies of the first, second and deep-in-bulk layers for different slab thicknesses in Fig. 2. Once again, for thickness greater than 10 the results tend to converge to the same value. From these considerations, the choice of a 20-layer slab proves to be thick enough to

avoid surface state hybridization, as well as adequately representing the results for even thicker slab geometries.

## FULL TOPOLOGICAL BANDGAP DESCRIPTION

The full information of the spectral weight distribution of the system is in principle given by the momentum-resolved spectral function

$$A(\mathbf{k}, \omega) = \frac{1}{\omega + \mu - H(\mathbf{k}) - \Sigma(\omega)}. \tag{16}$$

This quantity is however, in a DMFT-QMC scenario, of difficult analysis, because it involves the calculation, via analytical continuation on the real axis, of the full self-energy matrix. This process, involving techniques such as Pade or stochastic Maximum-Entropy, is in general not trivial when applied to the self-energy, and it proves especially difficult in our case which, as detailed in the previous section, is multi-orbital, multi-layer and contains off-diagonal and noisy components. Nevertheless, relevant information on the spectral weight distribution can be evinced from *local* spectral function $A(\omega)$, as discussed relatively to figure 3 in the main text, which is in general less cumbersome to treat through analytic continuation, involving diagonal components of the Green's function only.

Besides $A(\omega)$, the description of the spectral weight distribution near the Fermi level can benefit from an analysis of the topological bandgap of the effective Hamiltonian, highlighting the zero-energy quasiparticle excitations. This study can also address another issue: in our analytical derivation, we have up to now considered a finite system possessing only one surface, on which the effective Hamiltonian is $2 \times 2$. In a finite slab geometry such as the one employed in the main text, however, it is necessary to account for the presence of both surfaces to identify the positions in momentum space of all the exceptional points and Fermi arcs.

In Fig. 3 we show the value of the real bandgap between the surface gap-closing bands of energy $E_+$ and $E_-$ across all the Brillouin Zone. It is immediate to notice the presence of finite length Fermi Arcs, where the system is gapless. These originate and end at exceptional points of opposite vorticity. In an unperturbed scenario, the BHZ slab is gapless at the high-symmetry points $X$ and $Z$. If a purely imaginary perturbation is added, the Dirac point evolve into pairs of EPs, stretching

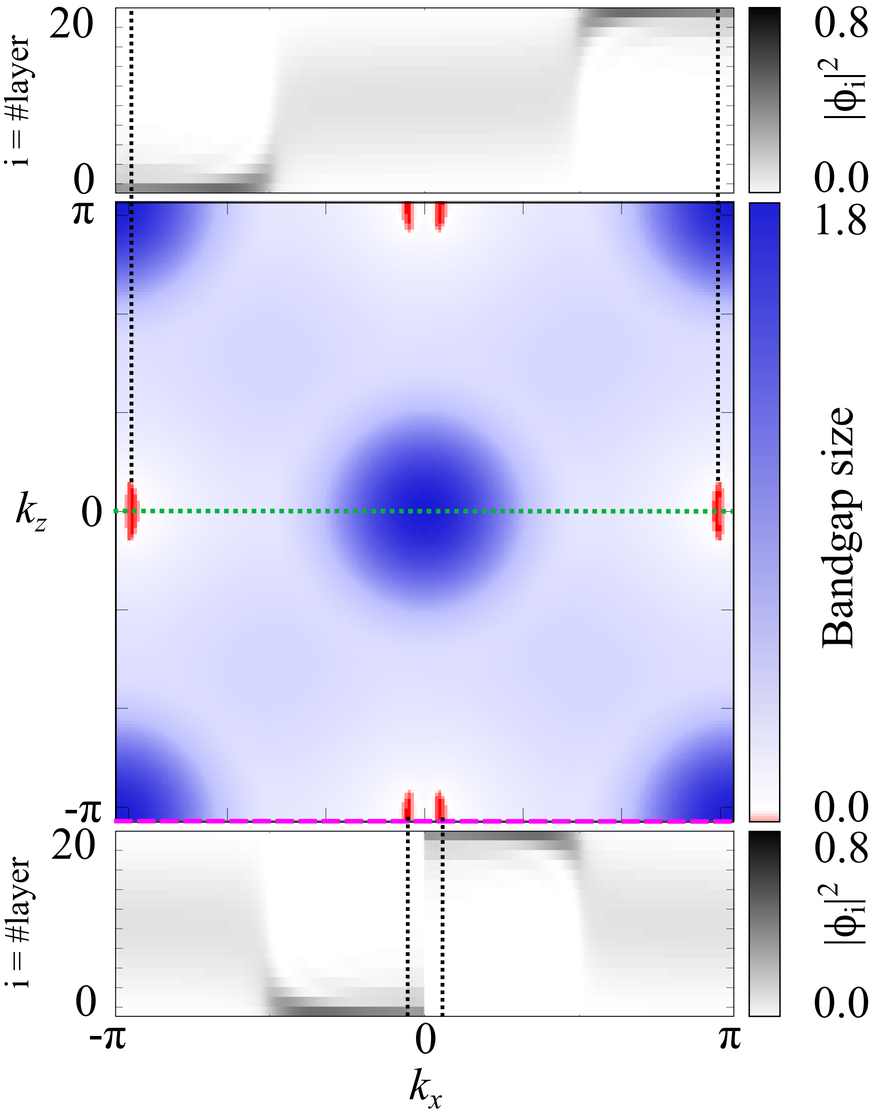


Figure 3. (color online) In the central panel of the plot the value of the real bandgap $|\mathrm{Re}(E_+ - E_-)|$ is plotted. The zero energy NH Fermi arcs are clearly visible. There are four arcs in total, two of which are localized on each surface, as it can be seen from the top and bottom panel. Here, the cumulative per-layer weight of the eigenvectors associated to $E_+$ (and equivalently $E_-$) are plotted, for fixed $k_z$ and varying $k_x$. The top panel refers to $k_z = 0$ (green dotted line in the central panel), the bottom one to $k_z = -\pi$ (purple dashed line). The $k_x$ position of the Fermi Arcs is highlighted by black dotted lines.

along the $k_z$ direction but still aligned with $X$ and $Z$. In presence of a finite Re$\Sigma$, however, a finite shift of the EPs in the perpendicular direction is expected, as mentioned in the main text. This turns out to affect the effective hamiltonians of the two surfaces in an opposite way, so that instead of two doubly-degenerate NH Fermi arcs we have now four non-degenerate ones. In the top and bottom panels of Fig. 3 we show the weight distribution of the eigenvectors associated to $E_+$ and $E_-$, resolved by layer. A slab of 20 layers is used, consistently with the main text. As it can be seen, at the location of the Fermi arcs, highlighted by vertical dotted lines, the states are overwhelmingly localized on opposite surfaces. Therefore, two Fermi arcs and 4 EPs are present on each surface of the slab, as expected from the analytical derivation.
